# Supplementary material for: Crown rupture during droplet impact on a dry smooth surface at increased pressure
Source: arXiv:2111.06066 source file (2021-11-11)
Supplement: Supplementary file 1 [file HighPressureImpact_SM.pdf]

# Crown rupture during droplet impact on a dry smooth surface at increased pressure: Supplementary Materials

Zhigang Xu, Longlong Wang, Tianyou Wang, and Zhizhao Che*

State Key Laboratory of Engines, Tianjin University, Tianjin, 300072, China.

November 11, 2021

## S1. Properties of the air at different environmental pressures

The properties of the air at different environmental pressures are obtained from the NIST reference fluid thermodynamic and transport properties database, NIST refprop, as listed in Table S1.

Table S1: Properties of the air at different environmental pressures at 20 °C.

| Pressure<br>$P$ (bar) | Density<br>$\rho$ (kg/m$^3$) | Dynamic viscosity<br>$\mu$ (mPa $\cdot$ s) | Mean free path<br>$\lambda$ (m) |
|---|---|---|---|
| 0.1 | 0.119 | 0.018 | $63.5 \times 10^{-8}$ |
| 0.5 | 0.595 | 0.018 | $12.7 \times 10^{-8}$ |
| 1 | 1.189 | 0.018 | $6.35 \times 10^{-8}$ |
| 2 | 2.378 | 0.018 | $3.17 \times 10^{-8}$ |
| 3 | 3.567 | 0.018 | $2.12 \times 10^{-8}$ |
| 4 | 4.756 | 0.018 | $1.59 \times 10^{-8}$ |
| 5 | 5.945 | 0.018 | $1.27 \times 10^{-8}$ |
| 6 | 7.134 | 0.018 | $1.06 \times 10^{-8}$ |
| 7 | 8.323 | 0.018 | $9.07 \times 10^{-9}$ |

## S2. Details of image processing

The size and the speed of the droplets were measured from the side-view images via an image processing algorithm using a customized Matlab program. After detecting the edges of the droplets from the brightness, the images were converted into binary images.

*Corresponding author, Email: chezhizhao@tju.edu.cn

After filling holes within the droplet area in the binary images, the total number of pixels $S$ and the centroid of the droplet $(x,\ y)$ can be obtained by using a customized Matlab program. Since the droplets are not exactly circular, the characteristic diameter of the droplet can be calculated by $D_0 = 2M\sqrt{S/\pi}$, where $M$ is the magnification factor obtained in a calibration procedure. The speed of the droplet impact can be calculated by $U = fM\,(y_1 - y_0)$, where $y_1$ and $y_0$ are the coordinates of the droplets' centroids on the two consecutive images just before the droplet impact, respectively, and $f$ is the camera's shooting frame rate.

The sizes and the number of the secondary droplets were measured from the bottom-view images via an image processing algorithm using a customized Matlab program. Briefly, after detecting the edges of the secondary droplets from the brightness, the images were converted into binary images. After filling holes within the areas of the secondary droplets in the binary images, the total number of pixels $S_1$ can be obtained. Since the secondary droplets are not exactly circular, the characteristic diameter of the secondary droplets can be calculated by $d{=}2M\sqrt{S_1/\pi}$. The diameters of all the outermost secondary droplets were measured after the liquid crown completely ruptures via an image processing algorithm.

## S3. Effects of the droplet size on the threshold pressure of splashing and the size of secondary droplets

The effect of the droplet size on the threshold pressure of splashing is shown in Fig. S1. As shown in Fig. S1, the threshold pressure of splashing decreases with increasing the size of the droplet. The "water hammer" effect can be used to explain the effect of the droplet size on the threshold pressure of splashing. For example, when the speed of the droplet impact is 2.3 m/s, the threshold pressure of splashing decreases with increasing the droplet size, and the threshold pressure of splashing is less than 1 bar. When the ratio between the destabilizing stress due to the gas $\Sigma_G$ and the stabilizing stress due to surface tension $\Sigma_L$ is 0.45 (i.e., $\Sigma_G/\Sigma_L{=}\sqrt{\gamma M_g}p\sqrt{\frac{D_0U}{4k_BT}}\frac{\nu_l}{\sigma} = 0.45$), the transition from the spreading to the splashing occurs (See Section IIID in the main text). Here we study the effect of the droplet size on the threshold pressure of splashing by varying the diameter of the droplet and the environmental pressure while fixing the other parameters. Thus, the threshold pressure of splashing decreases when we increase the size of the droplet.

The effect of the droplet size on the size of secondary droplets is shown in Fig. S2. The size of the secondary droplets increases with the initial droplet size, and the size of the secondary droplet increases with the environmental pressure.

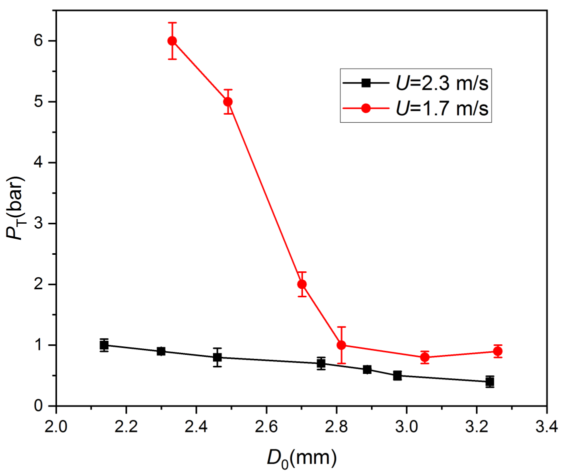


Figure S1: Effect of the droplet size on the threshold pressure of splashing.

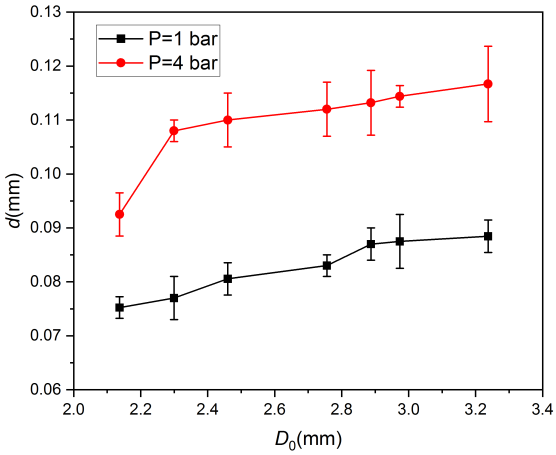


Figure S2: Effect of the initial droplet size on the size of secondary droplets. The speed of the droplet impact is 2.3 m/s.

## S4. Threshold pressure from the splash enhancement to the suppression of liquid crown

The effect of the environmental pressure on the diameter of the liquid crown is shown in Fig. S3. The diameter of the liquid crown $d_1$ is scaled by the initial diameter of the droplet $D_0$. As seen in Fig. S3, the diameter of the liquid crown increases first and then decreases with increasing the environmental pressure from 0.3 bar to 7 bar, and there are maximum diameters of the liquid crown at about 1 bar, indicating the threshold from the splash enhancement to the suppression of the liquid crown as the pressure increases. Therefore, the threshold from the splash enhancement to the suppression of liquid crown is about 1 bar when the Weber numbers of the droplet impact are 400 and 650.

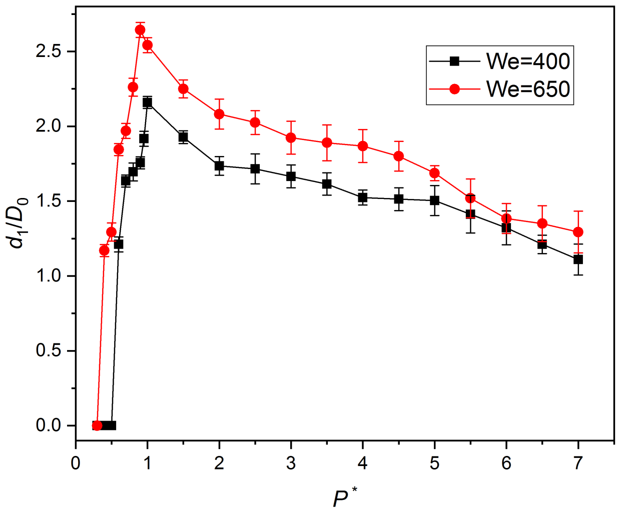


Figure S3: The effect of the environmental pressure on the diameter of the liquid crown. The diameter of the liquid crown $d_1$ is scaled by the initial diameter of the droplet $D_0$.
